# Supplementary material for: A Systematic Study of Data Modalities and Strategies for Co-training Large Behavior Models for Robot Manipulation
Source: arXiv:2602.01067 source file (2026-02-01)
Supplement: Supplementary file 1 [file appendix_preamble_arxiv.tex]

% --- Appendix formatting (portable) ---
\makeatletter

% If \appendices isn't defined (non-IEEE classes), fall back to \appendix
\providecommand{\appendices}{\appendix}

\renewcommand\appendices{%
  \par
  \setcounter{section}{0}%
  \setcounter{subsection}{0}%
  \setcounter{subsubsection}{0}%

  % Appendices sections use 1,2,3...
  \renewcommand{\thesection}{\arabic{section}}%
  % Subsections: 1A, 1B, ...
  \renewcommand{\thesubsection}{\thesection\Alph{subsection}}%
  % Subsubsections: 1A.1, 1A.2, ...
  \renewcommand{\thesubsubsection}{\thesubsection.\arabic{subsubsection}}%

  % Hyperref anchors (avoid collisions)
  \renewcommand{\theHsection}{apx.\arabic{section}}%
  \renewcommand{\theHsubsection}{apx.\arabic{section}\Alph{subsection}}%
  \renewcommand{\theHsubsubsection}{apx.\arabic{section}\Alph{subsection}.\arabic{subsubsection}}%

  % IEEE-only internal switch (guarded)
  \@ifundefined{@IEEEappendicestrue}{}{%
    \@IEEEappendicestrue
  }%
}
\makeatother

% Usage:
\clearpage
\appendices


% Reset figure/table counters and change numbering to S1, S2, ...
\setcounter{figure}{0}
\setcounter{table}{0}
\renewcommand{\thefigure}{S\arabic{figure}}
\renewcommand{\thetable}{S\arabic{table}}

% Fix hyperref anchors (so Fig. S1 doesn't link to Fig. 1)
\makeatletter
\renewcommand{\theHfigure}{apxfig.S\arabic{figure}}
\renewcommand{\theHtable}{apxtab.S\arabic{table}}
\makeatother
